# Supplementary material for: Tsunami Solitons Emerging from Superconducting Gap
Source: arXiv:2508.18311 ancillary file (2026-09-24)
Supplement: Supplementary file 1 [file readme.pdf]

# Mathematica code for generating Novikov equations

Daisuke A. Takahashi  
(Dated: September 7, 2025)

## I. CONTENT

The Mathematica notebook files provided here are used for generation of the (semi-)commuting pair of matrix differential operators and the Novikov equations following the procedure by Krichever (1977). The included files are:

- (i) Novikov-06.nb
- (ii) Novikov-06-KdV.nb ( $p, N$ ) = (2, 1)
- (iii) Novikov-06-NLS.nb ( $p, N$ ) = (1, 2)
- (iv) Novikov-06-Boussinesq-KK-SK.nb ( $p, N$ ) = (3, 1)
- (v) Novikov-06-ECSB.nb ( $p, N$ ) = (2, 2)

Novikov-06.nb is the most general file, and Novikov-06-\*.nb with \* = KdV, NLS, and Boussinesq-KK-SK are applications to the Korteweg-de Vries (KdV), nonlinear Schrödinger (NLS), and the Boussinesq, Kaup-Kupershmidt (KK), and Sawada-Kotera (SK) hierarchy.

Novikov-06-ECSB.nb is the most relevant file to the present work, where the hierarchy of equations considered in the main manuscript is generated. Here, ECSB means “extended coupled Schrödinger-Boussinesq”.

The value  $(p, N)$  implies that the seed operator  $\hat{L}$  [Eq. (1)] is a  $p$ -th order  $N \times N$  matrix differential operator. The default value in Novikov-06.nb is set to  $(p, N) = (2, 3)$ .

For readers who are familiar with the theory of hierarchy, Novikov-06-KdV.nb will be most illustrative, where the higher-order KdV equations are generated.

## II. SEMI-COMMUTING DIFFERENTIAL OPERATOR

We briefly summarize the concept of the semi-commuting differential operator. Let  $\hat{L}$  and  $\hat{M}$  be  $N \times N$  matrix differential operator ( $N \geq 1$ )

$$\hat{L} = \sum_{n=0}^p A^{(n)} \partial_x^n, \quad \hat{M} = \sum_{m=0}^q B^{(m)} \partial_x^m, \quad (1)$$

where  $p \geq 1$  and  $q \geq 0$ . We assume that the highest-order coefficient matrix of  $\hat{L}$  is diagonal, constant, full-rank, and nondegenerate, and the next highest one has no diagonal entries:

$$A_{i,j}^{(p)} = a_{i,i} \delta_{i,j}, \quad a_{i,i} \neq 0, \quad a_{i,i} \neq a_{j,j} \text{ if } i \neq j, \quad (2)$$

$$A_{i,i}^{(p-1)} = 0. \quad (3)$$

Let us write their commutator

$$[\hat{L}, \hat{M}] = \sum_{l=0}^{p+q} \text{Comm}^{(l)} \partial_x^l. \quad (4)$$

Then, we define that  $\hat{M}$  semi-commutes with  $\hat{L}$  if

$$\text{Comm}^{(l)} = \mathbf{0}_N, \quad l = p+1, p+2, \dots, p+q, \quad (5)$$

$$\text{Comm}_{i,i}^{(p-1)} = 0, \quad (6)$$

where  $\mathbf{0}_N$  is an  $N \times N$  zero matrix. Note that the concept of semi-commutativity is *not* symmetric with respect to  $\hat{L}$  and  $\hat{M}$ .

The above semi-commuting conditions (5) and (6) completely determines  $B^{(m)}$ 's; they are expressed by  $A^{(n)}$ 's, their derivatives  $A_x^{(n)}$ ,  $A_{xx}^{(n)}$ ,  $\dots$ , and several constants of integration. Using this result, the remaining  $\text{Comm}^{(l)}$ 's can all be expressed only by  $A^{(n)}$ 's and their derivatives. Hence, the full commuting condition  $[\hat{L}, \hat{M}] = 0$ , i.e.,

$$\text{Comm}^{(l)} = \mathbf{0}_N, \quad l = 0, 1, \dots, p-2, \quad (7)$$

$$\text{Comm}_{i,j}^{(p-1)} = 0, \quad (i \neq j), \quad (8)$$

now define the ordinary differential equations for  $A^{(n)}$ 's, which are the Novikov equations arising from the seed differential operator  $\hat{L}$ .

If we generalize the commuting condition to the Lax equation  $b\hat{L}_t = [\hat{L}, \hat{M}]$ , where  $b$  is nonzero constant, we obtain the time-evolution equations for  $A^{(n)}$ 's, defining a hierarchy of classical integrable equations. Furthermore, if  $p > q$ , the Zakharov-Shabat equation  $b\hat{L}_t - a\hat{M}_y = [\hat{L}, \hat{M}]$ , where  $a$  is a nonzero constant, defines a well-behaved (2+1)-dimensional integrable equation.

If some of the assumptions (2) and (3) do not hold but still a semi-commuting operator  $\hat{M}$  exists, the determination steps described below need a slight modification, which are not currently supported. For example, the sine-Gordon equation, where  $A^{(p)} = A^{(1)}$  is  $4 \times 4$  and  $a_{11} = 1$ ,  $a_{22} = -1$ ,  $a_{33} = a_{44} = 0$ , does not satisfy (2) [Takhtadzhyan-Faddeev (1974); see also arXiv:2301.08705].

## III. CODE FOR GENERATING NOVIKOV EQUATION

Here, we describe the content of Novikov-06.nb. We write  $p = \text{pmax}$ ,  $q = \text{qmax}$ , and  $N = \text{msize}$  in the file.

Step 1 — First compute the coefficient matrices for the commutator  $[\hat{L}, \hat{M}] = \sum_{l=0}^{p+q} \text{Comm}^{(l)} \partial_x^l$ . To do so, we prepare a temporary operand  $\phi = \phi_0 e^{kx}$  with  $\phi_0$  an  $x$ -independent vector and  $k$  the formal parameter, and determine  $\text{Comm}^{(l)}$ 's via the relation  $e^{-kx} [\hat{L}, \hat{M}] \phi = \sum_{l=0}^{p+q} \text{Comm}^{(l)} k^l \phi_0$ .

Step 2 — Determine the off-diagonal elements of  $B^{(m)}$ 's by imposing the condition that the off-diagonal elements of  $\text{Comm}^{(l)}$ 's vanish. More specifically, we solve the simultaneous equations  $\text{Comm}_{i,j}^{(l)} = 0$  for  $i \neq j$  and  $p \leq l \leq p+q$  with respect to the variables  $B_{i,j}^{(m)}$  for  $i \neq j$  and  $0 \leq m \leq q$ . The

solution is uniquely expressed in the form

$$B_{i \neq j}^{(m)} = P\left(A_{i,j}^{(n')}, B_{i,i}^{(m')}, \partial_x B_{i \neq j}^{(m'>m)}, \text{ and their derivatives}\right), \quad (9)$$

where the off-diagonal component  $B_{i \neq j}^{(m)}$ ,  $i \neq j$ , is briefly expressed as  $B_{i \neq j}^{(m)}$ , and  $P$  is a certain polynomial function. Henceforth (9) is used as a new definition of  $B_{i \neq j}^{(m)}$  in the code. Since the  $B_{i \neq j}^{(m'>m)}$ 's and their derivatives included in the above  $P$  can be eliminated via the definitions of the higher-order coefficients, all solutions can reduce to the form

$$B_{i \neq j}^{(m)} = \tilde{P}\left(A_{i,j}^{(n)}, B_{i,i}^{(m')}, \text{ and their derivatives}\right). \quad (10)$$

Step 3 — We next determine the diagonal components  $B_{i,i}^{(m)}$ 's. Let us impose  $\text{Comm}_{i,i}^{(l)} = 0$  for  $p-1 \leq l \leq p+q-1$  and solve them with respect to  $\partial_x B_{i,i}^{(m)}$ 's (not  $B_{i,i}^{(m)}$ 's themselves). The solution can be uniquely expressed by  $A_{i,j}^{(n)}$ 's and their derivatives, and furthermore, they have a form allowing the symbolic integration. So, we write the integration constant corresponding to  $B_{i,i}^{(m)}$  as  $b_{i,i}^{(m)}$ . Thus  $B_{i,i}^{(m)}$ 's are completely determined and expressed by  $A_{i,j}^{(n)}$ 's, their derivatives, and the constants  $b_{i,i}^{(m)}$ 's.

The remaining nonzero elements in the commutator  $[\hat{L}, \hat{M}]$ , that is,  $\text{Comm}_{i,j}^{(l)}$  with  $i \neq j, 0 \leq l \leq p-1$  and  $\text{Comm}_{i,i}^{(l)}$  with  $0 \leq l \leq p-2$ , are used to define the system of differential equation for  $A_{i,j}^{(n)}$ 's. If we require that all these components vanish, the resultant system is the Novikov equation, and  $\hat{L}$  and  $\hat{M}$  commute. If we assume that it is proportional to the

time derivative  $\hat{L}_t$ , we obtain the Lax equation which defines a time evolution.

The next ‘‘Step 3.5’’ is just a technical one, where  $B$ 's and  $\text{Comm}$ 's are re-defined based on the final result obtained in the above Step 3, in order to avoid repeating the same calculation.

In the remaining part of the code, several functions which make it easy to read the output of the computed operators are introduced. Note that the term-collecting functions in individual examples are slightly different, since  $b_{i,i}^{(m)}$  are re-parametrized in a way suitable for each problem. Furthermore, we provide the following ‘‘symmetrized’’ expression as below.

The last part of the file performs an optional procedure. We symmetrize the differential operator in the form  $\hat{L} = \sum_{n=0}^p \{\partial_x^n, \tilde{A}^{(n)}\}$  and  $\hat{M} = \sum_{m=0}^q \{\partial_x^m, \tilde{B}^{(m)}\}$ , which is useful in checking the self-adjointness and sometimes makes the expression much shorter. If  $i^n \tilde{A}^{(n)}$  are all hermitian, then  $\hat{L}$  is self-adjoint, and therefore its bounded eigenfunctions all have real eigenvalues, which strongly restrict the possible types of solitons. The relation between  $A^{(n)}$ 's and  $\tilde{A}^{(n)}$ 's are given by

$$A^{(j)} = \sum_{h=j}^p \left[ \binom{h}{j} + \delta_{hj} \right] \partial_x^{h-j} \tilde{A}^{(h)}, \quad (11)$$

$$\tilde{A}^{(j)} = \sum_{h=j}^p \frac{-(2^{h-j+1} - 1)B_{h-j+1}}{h+1} \binom{h+1}{h-j+1} \partial_x^{h-j} A^{(h)}, \quad (12)$$

for  $j = 0, 1, \dots, p$ , where  $B_j$  is the Bernoulli number (not to be confused with  $B^{(j)}$ ). The same relation for  $\hat{M}$  also follows by replacing the letter  $A$ ,  $p$  to  $B$ ,  $q$ .
